# Supplementary material for: Universal Correlations in Local Measurements Directly Probe Effective Diffusivity
Source: arXiv:2308.08595 ancillary file (2026-08-05)
Supplement: Supplementary file 1 [file SM.pdf]

# Supplemental Material for: “Universal Fluctuations of Local Measurement in Low-Dimensional Systems”

Omer Granek<sup>1</sup>

<sup>1</sup>*Department of Physics, Technion-Israel Institute of Technology, Haifa, 3200003, Israel.*

## CONTENTS

|                               |   |
|-------------------------------|---|
| Simulation details            | 1 |
| A. Setup and protocol         | 1 |
| B. Integration scheme         | 1 |
| C. Steady-state distributions | 2 |
| D. Measurement procedure      | 4 |
| References                    | 4 |

## SIMULATION DETAILS

### A. Setup and protocol

In each realization of the models, a periodic system  $[-L/2, L/2]$  containing  $N = \rho_0 L$  particles is initialized at time  $t = t_i < 0$  in a random configuration. The particles are then allowed to evolve until time  $t = 0$ . The integration scheme employed is detailed in Section B. The convergence to a steady state in the vicinity of the probe is verified against the analytical expressions known in the literature, as described in Section C.

Between  $t = 0$  and  $t = t_f$ , the time-averaged signals  $\bar{A}(t) = \bar{\mathcal{P}}(t), \bar{V}(t), \bar{F}(t), \bar{P}(t)$  are measured as described in Section D. The ensemble averages  $\langle \bar{A}(t) \rangle$  and  $\langle \bar{A}^2(t) \rangle_c = \langle \bar{A}^2(t) \rangle - \langle \bar{A}(t) \rangle^2$  are then computed from  $M$  realizations of the simulation. Model parameters:  $\rho_0 = v = \mu = \alpha = T = 1, L = 10^4$ . I:  $U_0 = 30, b = 3$ . II-III (respectively):  $V_0 = 0.25, 7.5, b_- = 0.26, 1.25, b_+ = 0.74, 8.75, \ell = 1, 5$ . IV:  $\chi = 0.5$ . Protocol parameters (respectively I-IV):  $t_i = -10^5, -10^5, -2 \cdot 10^6, -10^8, M/10^3 = 2.5, 2, 3.5, 6$  and  $t_f = 10^5$  (all).

### B. Integration scheme

*Model I* — Equation (3) is integrated using Eulerian time stepping. The position of a Brownian particle  $x_n(t_{i+1})$  at time  $t_{i+1} = t_i + \Delta t$  is given by

$$x_n(t_{i+1}) = x_n(t_i) - \mu U' [x_n(t_i)] \Delta t + \sqrt{2\mu T \Delta t} \eta_n(t), \quad (\text{S.1})$$

where  $\eta_n(t_i) \sim \mathcal{N}(0, 1)$  are i.i.d and  $\Delta t = 10^{-2}$ . In practice, the wall potential is centered at  $x = 0$  instead of  $x = \pm L/2$ . Specifically, Eq. (S.1) is integrated with  $x_n \rightarrow x_n + L/2$ . The shift is also applied to all measured

observables. Due to the periodic boundary conditions, the shifted system is equivalent to the original one.

*Model II* — Equation (4) is integrated using Eulerian time stepping. The position of an active run-and-tumble particle  $x_n(t_{i+1})$  at time  $t_{i+1} = t_i + \Delta t_i$ , with  $\Delta t_i = \Delta t = 10^{-2}$  by default, is given by

$$v_n(t_i) = v u_n(t_i) - \mu V'(x_n(t_i)), \quad (\text{S.2})$$

$$x_n(t_{i+1}) = x_n(t_i) + v_n(t_i) \Delta t_i, \quad (\text{S.3})$$

where  $u_n(t_i)$  is the particle orientation. The time stepping is further modified by an adaptive mesh-refinement procedure detailed below. The procedure leads to an exact integration of Eq. (4) up to machine precision.

The internal degree of freedom  $u_n(t_i) = \pm 1$  is updated according to a continuous-time Monte Carlo scheme. At time  $t_0 = 0$ , a flipping time  $\tau_0 \sim \text{Exp}(2/\alpha)$  is drawn. For all  $i > 1$ , if  $\tau_0 \in [t_i, t_{i+1})$ , then flipping occurs in this interval and  $u_n(t_{i+1}) = -u_n(t_i)$ . The flipping time is then updated to  $\tau_1 = \tau_0 + \delta\tau$ , where  $\delta\tau \sim \text{Exp}(2/\alpha)$  is drawn independently of  $\tau_0$ . If a flipping event did not occur,  $u_n(t_{i+1}) = u_n(t_i)$ .

The adaptive mesh-refinement procedure is detailed as follows. If a flipping event has occurred at  $\tau_0 \in [t_i, t_{i+1})$ , then the interval is split at the flipping time  $t_i + \tau_0$ . The integration of Eqs. (S.2)-(S.3) is then performed separately over the intervals  $[t_i, t_i + \tau_0)$  and  $[t_i + \tau_0, t_{i+1})$ , with the flipping  $u(t_i + \tau_0) = -u(t_i)$  being applied in between. Similar refinement is applied to account for transitions between the different constant-force regions depicted in Fig. 1(b). The boundaries of these regions are denoted by  $\{X_j\}$ . If at a given integration step,  $X_j \in [x_n(t_i), x_n(t_{i+1}))$ , then the time-interval is cut at the transition time  $t_i + |X_j - x_n(t_i)|/v_n(t_i)$ . Once more, the integration of Eqs. (S.2)-(S.3) is performed over each interval separately, with the velocity  $v_n(t_i + \tau_0)$  being updated according to the shift in the constant force value.

*Model III* — Equation (5) is integrated using Eulerian time stepping. The position of a Brownian particle  $x_n(t_{i+1})$  at time  $t_{i+1} = t_i + \Delta t_i$  is given by

$$x_n(t_{i+1}) = x_n(t_i) - \mu V' [x_n(t_i) + b_- w_n(t_i)] \Delta t_i + \sqrt{2\mu T \Delta t_i} \eta_n(t), \quad (\text{S.4})$$

where  $w_n(t_i) = [1 + u_n(t_i)]/2$ . The above update rule for  $u_n(t_i)$  and the adaptive mesh-refinement due to flipping are implemented. However, due to the irregularity of Brownian motion, no refinement is used for constant-

force region transitions.

*Model IV* — The model is a variant of the binomial experiment. It is simulated by summing independent and biased coin flips. The position  $x_n(t_{i+1})$  of a random walker at time  $t_{i+1} = t_i + 1$  ( $\Delta t = 1$ ) is given by

$$x_n(t_i) = x_n(t_i) + \xi_n(t_i), \quad (\text{S.5})$$

where  $\xi_n(t_i) = \pm 1$  with probability  $(1 \pm \chi \delta_{x_n(t_i), 0})/2$ .

### C. Steady-state distributions

In Models II-III, the time-dependent particle distribution is  $\rho(x, u, t) = NP(x, u, t)$ , where  $P(x, u, t)$  is the time-dependent probability density. Importantly, the particle density  $\rho(x, t) \equiv \sum_u \rho(x, u, t)$  is a conserved field, while the magnetization  $m(x, t) \equiv \sum_u u \rho(x, u, t)$  is not. Therefore,  $\rho(x, t)$  is the slowest mode in the system. In Models I and IV, it is the only mode in the system. The convergence to the steady state in all four models can thus be verified by comparing the average particle density profile at time  $t = 0$  to the analytical expressions for the steady-state density  $\rho_s(x)$  known in the literature (see Fig. 1), which are reviewed below.

*Model I* — Since the system is at equilibrium,  $\rho_s$  is given by the Boltzmann distribution as

$$\rho_s(x) = \rho_0 e^{-\beta U(x)}, \quad (\text{S.6})$$

where  $\beta = 1/T$ . Equation (S.6) is seen to agree with the measured density profile in Fig. 1(a). Note that,  $\rho_s(\pm L/2) = \rho_0 e^{-\beta U_0}$ . For the chosen parameters  $U_0 = 30$  and  $\beta = 1$ , this provides  $\rho_s(\pm L/2)/\rho_0 = e^{-30} \simeq 0$ . Likewise, the Arrhenius time to escape over the potential barrier is  $\simeq e^{\beta U_0} = e^{30} \gg t_f$ . Hence, the walls are effectively impenetrable throughout the simulation duration. However, as stated in the main text, the equations of state and the results remain identical even for penetrable walls with small  $\beta U_0$ .

*Model II* — For one-dimensional run-and-tumble particles, the steady-state density in an infinite system is given by the explicit formula [1, 2]

$$\rho_s(x) = \frac{\rho_L}{1 - [\frac{\mu}{v} V'(x)]^2} \exp \left\{ - \int_{-\ell/2}^x dy \frac{\beta_{\text{eff}} V'(y)}{1 - [\frac{\mu}{v} V'(y)]^2} \right\}, \quad (\text{S.7})$$

where  $\beta_{\text{eff}} = 1/T_{\text{eff}}$ ,  $T_{\text{eff}} \equiv \mu\alpha/v^2$  is the effective temperature and  $\rho_L = \rho_s(x < -\ell/2)$  and  $\rho_R = \rho_s(x > \ell/2)$  respectively are the density to the probe's left and right, such that the average background density is

$$\rho_0 = \lim_{L \rightarrow \infty} \int_{-L/2}^{L/2} \frac{dx}{L} \rho_s(x) = \frac{\rho_R + \rho_L}{2}. \quad (\text{S.8})$$

The corresponding average net force exerted on the particles is given by [3–5]

$$\langle F \rangle = - \int dx \rho_s(x) V'(x) = T_{\text{eff}} (\rho_R - \rho_L), \quad (\text{S.9})$$

where the second equality, which can be identified as an effective ideal gas equation of state, stems from  $-V' \rho_s = T_{\text{eff}} \partial_x \exp(-\beta_{\text{eff}} V_{\text{eff}})$ . Upon inserting Eq. (S.7), Eq. (S.9) becomes

$$\langle F \rangle = 2T_{\text{eff}} \rho_0 \tanh \frac{\Delta V_{\text{eff}}}{2T_{\text{eff}}}, \quad (\text{S.10})$$

$$\Delta V_{\text{eff}} \equiv \int_{-\ell/2}^x dy \frac{V'(y)}{1 - [\frac{\mu}{v} V'(y)]^2}. \quad (\text{S.11})$$

For a periodic system of size  $L \gg \ell, v/\alpha, |x|$ , the constant diffusive current in the system, which scales as  $L^{-1}$ , leads to a correction of  $\mathcal{O}(L^{-1})$  to Eq. (S.7) [6]. For this model, to expedite the relaxation and reduce computation time, the system is initialized at time  $t = t_i < 0$  at a random configuration drawn from Eq. (S.7) instead of a uniform distribution. As seen in Fig. 1(b), the simulation protocol is sufficient for the distribution at  $t = 0$  to be indistinguishable from Eq. (S.7). To verify that the change in initial distribution does not affect the results, a uniform initial distribution is also used for a smaller system (see Fig. 2).

*Model III* — The steady state density current  $J$  in the Ajdari-Prost model is [7, 8]

$$J = \mu [-T \partial_x - V'_{\text{eff}}(x)] \rho_s(x). \quad (\text{S.12})$$

The effective potential  $V_{\text{eff}}(x)$  for the variant of the model used here is given by

$$V_{\text{eff}}(x) \equiv \bar{V}(x) + \int_{-\ell/2-b_-}^x dx p_s(x) \delta V'(x), \quad (\text{S.13})$$

where  $\bar{V}(x) \equiv \sum_u V(x + (1+u)b_-/2)$ ,  $\delta V(x) \equiv \sum_u u V(x + (1+u)b_-/2)$  and  $p_s(x) \equiv m_s(x)/\rho_s(x)$  and  $m_s$  respectively are the steady-state polarization and magnetization fields. In an infinite system, for which  $J = 0$ , the steady-state density is thus

$$\rho_s(x) = \rho_L \exp[-\beta V_{\text{eff}}(x)], \quad (\text{S.14})$$

where  $\rho_L \equiv \rho(x < -\ell/2 - b_-)$ . As in Model II, the potential form of the solution implies the ideal gas equation of state

$$\langle F \rangle = - \sum_{u=\pm 1} \int dx \rho_s(x, u) \partial_x V \left( x + \frac{1+u}{2} b_- \right) \quad (\text{S.15})$$

$$= \int dx \rho_s \partial_x V_{\text{eff}} = T(\rho_R - \rho_L), \quad (\text{S.16})$$

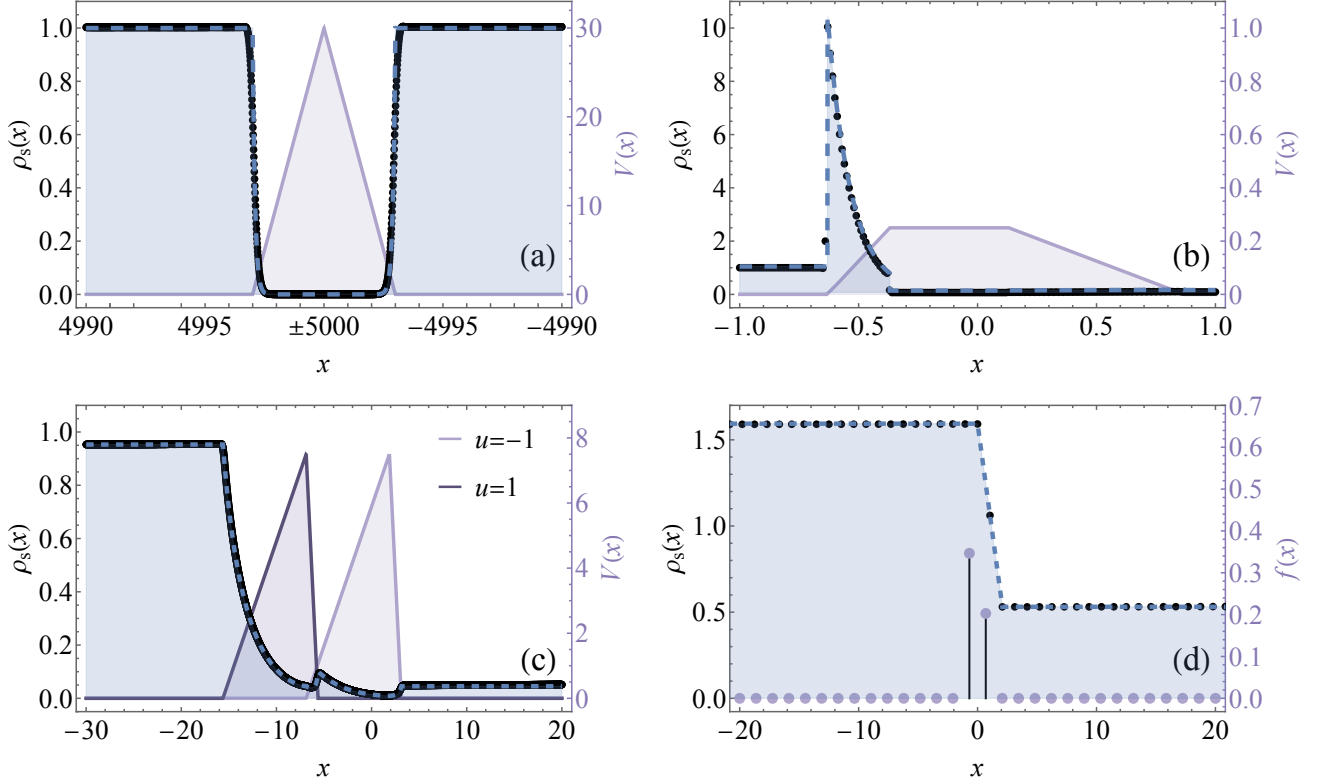

Figure 1. Steady-state density  $\rho_s(x)$  for Models I-IV (respectively, (a-d)): simulation protocol (symbols) and theory (dashed lines). The density profile is overlayed by: (a-b) the potential landscape  $V(x)$ , (c)  $V[x + b_-(1+u)/2]$  where  $u = \pm 1$  and (d) force landscape  $f(y \leftrightarrow z)$  with  $y = x \pm 1/2$  and  $z = x \mp 1/2$  (respectively), plotted for  $x = 1/2 + k$ , with  $k$  an integer. See text for comparison details and parameters.

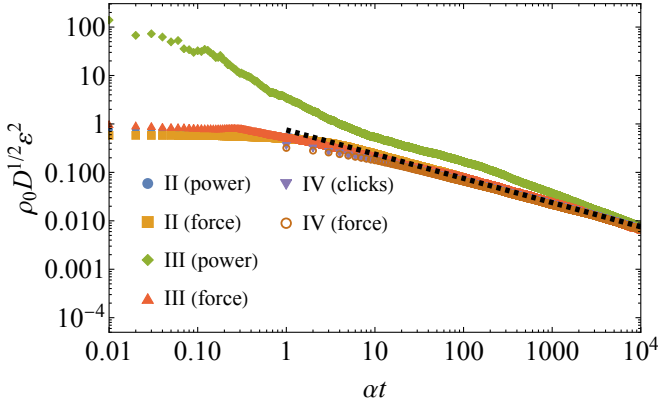

Figure 2. Reproduction of Fig. 1(e) (Models II-IV) for a smaller system ( $L = 10^3$ ). Here,  $t_i = -10^6$ ,  $t_f = L = 10^3$  and  $M/10^3 = 4, 2, 6$  (reseptively II-IV). See Fig. 1 for a description and additional parameters.

where  $\rho_R \equiv \rho(x > \ell/2)$  and the second equality follows from Eq. (S.13). Similarly to the run-and-tumble case, for a periodic system of size  $L \gg \ell, |x|$ , the constant diffusive current  $J \sim L^{-1}$  provides an  $\mathcal{O}(L^{-1})$  correction to Eq. (S.14). Once more, in Fig. 1(c), the simulation pro-

tol is seen to be sufficient for the distribution at  $t = 0$  to be indistinguishable from Eq. (S.14). To perform the comparison,  $p_s = m_s/\rho_s$  is computed from the measured data. The integral in Eq. (S.13) is then evaluated numerically, from which  $\rho_s$  is obtained via Eq. (S.14). The results in Fig. 1 for this model are also reproduced in a smaller system (see Fig. 2).

*Model IV* — As in Models II-III, in an infinite system, for which the current vanishes, the solution is potential and is given by Eq. (S.14). Here, the mobility is set without loss of generality to unity so that  $T = D = 1/2$ . The effective potential  $V_{\text{eff}}(x)$  in the model can be determined via the heat released during the transition  $x \rightarrow x'$ ,  $|x - x'| = 1$ , as [9]

$$V_{\text{eff}}(x) - V_{\text{eff}}(x') = T \ln \frac{p(x \rightarrow x')}{p(x' \rightarrow x)}, \quad (\text{S.17})$$

where the transition probability is

$$p(x \rightarrow x') = (1 \pm \delta_{x,0} \delta_{x',\pm 1} \chi)/2. \quad (\text{S.18})$$

Setting without loss of generality  $V_{\text{eff}}(-\infty) = -\ln(1-\chi)$  provides

$$V_{\text{eff}}(x) = \frac{1}{2} \begin{cases} -\ln(1+\chi), & x \geq 1 \\ 0, & x = 0 \\ -\ln(1-\chi), & x \leq -1 \end{cases}. \quad (\text{S.19})$$

The force  $f(x \leftrightarrow x + \Delta x) = -\Delta V_{\text{eff}}/\Delta x$ , where  $\Delta V_{\text{eff}} \equiv V_{\text{eff}}(x + \Delta x) - V_{\text{eff}}(x)$  and  $\Delta x = \pm 1$ , is then given by

$$f(x \leftrightarrow x') = \frac{1}{2} \begin{cases} \pm \ln(1 \pm \chi), & 0 \leftrightarrow \pm 1 \\ 0, & \text{otherwise} \end{cases}. \quad (\text{S.20})$$

Plugging Eq. (S.19) and  $\beta = 2$  into Eq. (S.6) then leads to

$$\rho_s(x) = \rho_0 \begin{cases} 1 + \chi & x \geq 1 \\ 1 & x = 0 \\ 1 - \chi & x \leq -1 \end{cases}, \quad (\text{S.21})$$

which agrees with the numerically-measured profile (see Fig. 1(d)). In the steady state, the average clicks signal by the detector at  $x = 0$  is given by  $\langle C \rangle = \rho_s(0) = \rho_0$ . The average net force is given by

$$\langle F \rangle = \sum_n \langle f[x(t) \leftrightarrow x(t+1)] \rangle \quad (\text{S.22})$$

$$= \sum_{xx'} f(x \leftrightarrow x') p(x' \rightarrow x) \rho_s(x'). \quad (\text{S.23})$$

where the second equality follows from time-translation invariance. Inserting Eqs. (S.18), (S.20) and (S.21) into Eq. (S.23) then yields

$$\langle F \rangle = \frac{\rho_0}{2} [(1+\chi) \ln(1+\chi) - (1-\chi) \ln(1-\chi)]. \quad (\text{S.24})$$

#### D. Measurement procedure

Each local measurement  $A = \mathcal{P}, \mathcal{V}, F, \mathcal{P}, C$  is given by  $A(t_i) = \sum_n a(x_n(t_i), u_n(t_i))$ , where  $a(x_n(t_i), u_n(t_i))$  are given by Eq. (6), the summands in Eqs. (6-7) and the expressions for  $C(t)$ ,  $\mathcal{P}(t)$  and  $\mathcal{V}(t)$  that follow. The time-averaged signal is computed as

$$\bar{A}(t_i) = \frac{1}{t_i} \sum_{j=0}^{i-1} \Delta t_j \sum_n a_n(t_j). \quad (\text{S.25})$$

For  $A = \mathcal{P}$ , the velocity is discretized such that  $a_n(t_j) = [x_n(t_{j+1}) - x_n(t_j)] f_n(t_j)$  (Models II and IV). For Model III, due to the overdamped Langevin dynamics, the physical heat release is provided by the Stratonovich discretization [9]. Specifically,  $\Delta t_j a_n(t_j) = [x_n(t_{j+1}) - x_n(t_j)][f_n(t_{j+1}) + f_n(t_j)]/2$ .

The above analytic expressions are then compared to

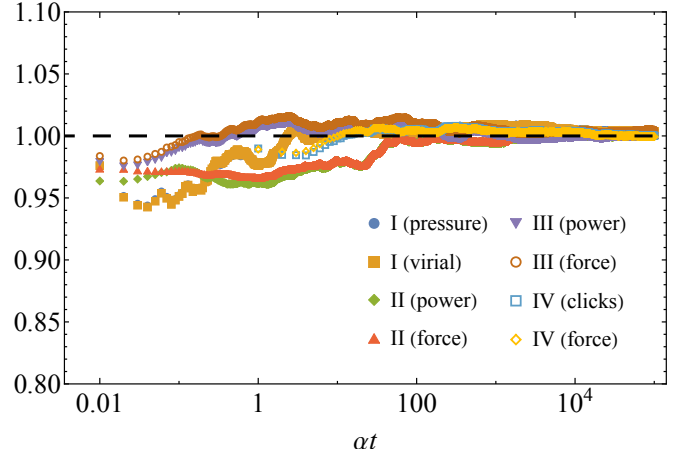

Figure 3. Comparison of the measurements of  $A = \mathcal{P}, \mathcal{V}, F, \mathcal{P}, C$  to their respective steady-state values:  $\langle \bar{A}(t) \rangle / \langle A \rangle_{\text{th}}$  (all except  $A = \mathcal{P}$ ) and  $\langle \bar{A}(t) \rangle / \langle \bar{A}(t_f) \rangle$  ( $A = \mathcal{P}$ ). Here,  $\langle A \rangle_{\text{th}}$  is the analytic expression, i.e.  $\langle \mathcal{P} \rangle_{\text{th}} = \rho_0 T$ ,  $\langle \mathcal{V} \rangle_{\text{th}} = -\rho_0 L T / 2$  and Eqs. (S.9), (S.16) and (S.24). For Eq. (S.16),  $\rho_R$  and  $\rho_L$  are computed by averaging  $\rho_s(x)$  profile in Fig. 1(c) over the regions where the potential vanishes.

$\langle \bar{A}(t) \rangle$ , with  $A = \mathcal{P}, \mathcal{V}, F, C$  in Fig. 3. The measurements for  $A = \mathcal{P}$  are compared to  $\langle \bar{A}(t_f) \rangle$  in the same figure. The agreement improves over time as further data are accumulated.

- 
- [1] K. Kitahara, W. Horsthemke, and R. Lefever, *Phys. Lett. A* **70**, 377 (1979).
  - [2] A. P. Solon, Y. Fily, A. Baskaran, M. E. Cates, Y. Kafri, M. Kardar, and J. Tailleur, *Nat. Phys.* **11**, 673 (2015), [arXiv:1412.3952](#).
  - [3] L. Angelani and R. D. Leonardo, *New J. Phys.* **12**, 113017 (2010).
  - [4] S. A. Mallory, C. Valeriani, and A. Cacciuto, *Phys. Rev. E* **90**, 032309 (2014), [arXiv:1407.3418](#).
  - [5] N. Nikola, A. P. Solon, Y. Kafri, M. Kardar, J. Tailleur, and R. Voituriez, *Phys. Rev. Lett.* **117**, 098001 (2016), [arXiv:1512.05697](#).
  - [6] O. Granek, Y. Kafri, and J. Tailleur, *Phys. Rev. Lett.* **129**, 038001 (2022), [arXiv:2108.11970](#).
  - [7] J. Prost, J.-F. Chauwin, L. Peliti, and A. Ajdari, *Phys. Rev. Lett.* **72**, 2652 (1994).
  - [8] F. Jülicher, A. Ajdari, and J. Prost, *Rev. Mod. Phys.* **69**, 1269 (1997).
  - [9] N. Shiraishi, *An Introduction to Stochastic Thermodynamics: From Basic to Advanced* (Springer Singapore, 2023).
